# Supplementary material for: Direct observation of exchange-driven spin interactions in one-dimensional system
Source: arXiv:1707.04575 source file (2017-07-14)
Supplement: Supplementary file 1 [file SI_foc_YAN.pdf]

# Supplementary information: direct observation of exchange-driven spin interactions in one-dimensional system

Chengyu Yan,[1,2,a)] Sanjeev Kumar,[1,2] Kalarikad Thomas,[1,2,b)] Michael Pepper,[1,2] Patrick See,[3] Ian Farrer,[4,c)] David Ritchie,[4] J. P. Griffiths,[4] and G. A. C. Jones[4]
[1)] *London Centre for Nanotechnology, 17-19 Gordon Street, London WC1H 0AH, United Kingdom*
[2)] *Department of Electronic and Electrical Engineering, University College London, Torrington Place, London WC1E 7JE, United Kingdom*
[3)] *National Physical Laboratory, Hampton Road, Teddington, Middlesex TW11 0LW, United Kingdom*
[4)] *Cavendish Laboratory, J.J. Thomson Avenue, Cambridge CB3 OHE, United Kingdom*

(Dated: 4 July 2017)

## I. SWAPPING THE INJECTOR AND DETECTOR

To further support the argument that the splitting of odd-numbered focusing peaks is not due to disorder, we exchange the role of the injector and detector as shown in supplementary Fig. 1. Due to the reversal of the focusing trajectory, the focusing spectrum occurs at the negative magnetic field end. However, it is important to notice that the splitting of first peak and lack of splitting of the second peak remain preserved. The peak splitting after swapping is ∼5.4 mT, almost identical to the value (5.5 mT) before swapping. This confirms the peak splitting is a result of 2D property, i.e SOI.

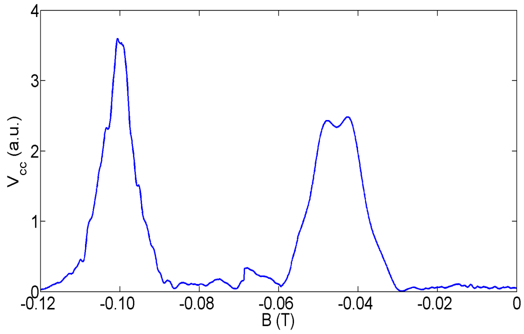


Supplementary Fig 1. **Representative result after swapping the injector and detector.** It is seen that the splitting of first peak and lack of splitting of the second peak remain preserved.

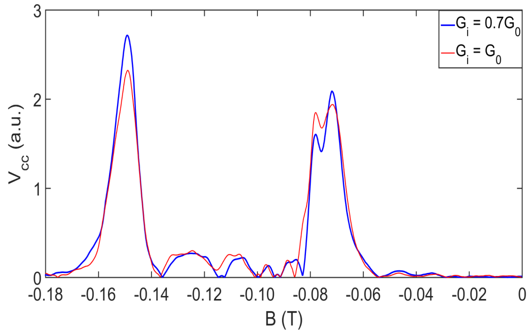


Supplementary Fig 2. **Representative result with linear focusing geometry.** The injector is set to $0.7G_0$ and $G_0$, respectively. The detector is fixed at $G_0$. The first peak shows pronounced splitting while the splitting is absent for the second peak.

## II. DISCUSSION ON THE ELECTRON BRANCHING

It is pointed out that disorder induced electron branching in the 90° geometry may result in the splitting of focusing peak[1], the sub-peaks produced thereby may not be relevant to the spin states. We argue that our results are not due to electron branching.

First, electron branching induced peak splitting remained preserved up to high injector conductance, e.g. the splitting is still observable at injector conductance of $5 \times \frac{2e^2}{h}$ as shown in Fig. 4(b) of Ref. 1. This can be understood from the semi-classical picture that increasing the injector conductance enlarges the injection angle span. Thus if a disorder is located along the focusing trajectory, it is more likely to cause scattering. This is quite different from our result where we observed that the peak splitting smears out rapidly when the injector conductance exceeds $2 \times \frac{2e^2}{h}$.

Second, the intensity of sub-peaks does not necessary become symmetric at the conductance plateau if the peak splitting arises from the disorder-induced electron branching as shown in Ref. 1. Our result reveals that the two sub-peaks, representing the two spin states, almost have identical intensity at conductance plateau which is

[a)] Electronic mail: uceeya3@ucl.ac.uk
[b)] Currently at Department of Physics, Central University of Kerala, Riverside Transit Campus, Padannakkad, Kerala 671314, India.
[c)] Currently at Department of Electronic and Electrical Engineering, University of Sheffield, Mappin Street, Sheffield S1 3JD, United Kingdom.

consistent with the theoretical calculation[2–4].

Third, we performed the focusing experiment with conventional linear geometry[5] on the same wafer which was used for the 90° geometry. Despite a change in the focusing periodicity (which is due to the variation in the separation between the injector and detector), the result is similar to that obtained from the 90° geometry as shown in supplementary Fig. 2. The first peak shows pronounced splitting while the splitting is absent for the second peak. Similarly the sub-peaks become symmetric when $G_i = G_0$ and asymmetric at $G_i = 0.7\ G_0$.


[1] D. Maryenko , F. Ospald, K. v. Klitzing, J. H. Smet, J. J. Metzger, R. Fleischmann , T. Geisel, V. Umansky *Phys. Rev. B* **85**, 195329 (2012).

[2] C.-K. Wang & K.-F. Berggren *Phys. Rev. B* **54**, R14257–R14260 (1996).

[3] C.-K. Wang & K.-F. Berggren *Phys. Rev. B* **57**, 4552–4556 (1998).

[4] D. J. Reilly, T. M. Buehler, J. L. O'Brien, A. R. Hamilton, A. S. Dzurak, R. G. Clark, B. E. Kane, L. N. Pfeiffer & K. W. West *Phys. Rev. Lett.* **89**, 246801 (2002).

[5] H. van Houten, C. W. J. Beenakker, J. G. Williamson, M. E. I. Broekaart, P. H. M. van Loosdrecht, B. J. van Wees, J. E. Mooij, C. T. Foxon, J. J. Harris *Phys. Rev. B* **39**, 8556–8575 (1989).
